# Supplementary material for: A User Centric Group Authentication Scheme for Secure Communication
Source: arXiv:2512.03551 source file (2025-12-03)
Supplement: Supplementary file 1 [file Appendix_SR.pdf]

## A Scyther Code Example

Here we provide the Scyther input code used for the formal analysis.

```
usertype Xid;
usertype Vec;
usertype SetS;
usertype Scalar;

function Acoeff;     /* Acoeff(x, S) -> Scalar */
function MulSV;      /* MulSV(Scalar, Vec) -> Vec */
function IP;         /* IP(Vec, Vec) -> Scalar */
function Agg;        /* Agg(Scalar, Scalar) -> Scalar */
function MulScalar;  /* MulScalar(Scalar, Scalar) -> Scalar */

/* One shared group key */
const kGrp;
/* Mark it secret (global) */
secret kGrp;

protocol GroupAuth3(U1, U2, U3, GM)
{
  role GM
  {
    fresh x1: Xid;
    fresh x2: Xid;
    fresh x3: Xid;
    fresh S: SetS;
    fresh g: Vec;
    fresh v: Vec;
    fresh f0: Scalar;

    send_0(GM, U1, x1, S, g);
    send_1(GM, U2, x2, S, g);
    send_2(GM, U3, x3, S, g);

    var M1: Scalar;
    var M2: Scalar;
    var M3: Scalar;

    recv_3(U1, GM, { M1 }kGrp);
    recv_4(U2, GM, { M2 }kGrp);
    recv_5(U3, GM, { M3 }kGrp);

    match(Agg(Agg(M1, M2), M3), MulScalar(IP(v, g), f0));
```

```
  claim(GM, Alive);
  claim(GM, Weakagree);
  claim(GM, Niagree);
  claim(GM, Nisynch);
  claim(GM, Secret, Agg(Agg(M1, M2), M3));
}

role U1
{
  var x1: Xid;
  var S: SetS;
  var g: Vec;

  recv_0(GM, U1, x1, S, g);

  fresh B1: Vec;
  var A1: Scalar;
  match(A1, Acoeff(x1, S));

  var Scaled1: Vec;
  match(Scaled1, MulSV(A1, B1));

  var M1: Scalar;
  match(M1, IP(Scaled1, g));

  send_3(U1, GM, { M1 }kGrp);

  claim(U1, Secret, B1);
  claim(U1, Alive);
  claim(U1, Weakagree);
  claim(U1, Niagree);
  claim(U1, Nisynch);
}

role U2
{
  var x2: Xid;
  var S: SetS;
  var g: Vec;

  recv_1(GM, U2, x2, S, g);

  fresh B2: Vec;
  var A2: Scalar;
  match(A2, Acoeff(x2, S));
```

```
    var Scaled2: Vec;
    match(Scaled2, MulSV(A2, B2));

    var M2: Scalar;
    match(M2, IP(Scaled2, g));

    send_4(U2, GM, { M2 }kGrp);

    claim(U2, Secret, B2);
    claim(U2, Alive);
    claim(U2, Weakagree);
    claim(U2, Niagree);
    claim(U2, Nisynch);
  }

  role U3
  {
    var x3: Xid;
    var S: SetS;
    var g: Vec;

    recv_2(GM, U3, x3, S, g);

    fresh B3: Vec;
    var A3: Scalar;
    match(A3, Acoeff(x3, S));

    var Scaled3: Vec;
    match(Scaled3, MulSV(A3, B3));

    var M3: Scalar;
    match(M3, IP(Scaled3, g));

    send_5(U3, GM, { M3 }kGrp);

    claim(U3, Secret, B3);
    claim(U3, Alive);
    claim(U3, Weakagree);
    claim(U3, Niagree);
    claim(U3, Nisynch);
  }
}
```
